# Supplementary material for: Real-Time Global Illumination Using OpenGL And Voxel Cone Tracing
Source: arXiv:2104.00618 source file (2021-04-01)
Supplement: Supplementary file 2 [file AppendixTemplate.tex]

% Appendix Template

\chapter{Appendix Title Here} % Main appendix title

\label{AppendixX} % Change X to a consecutive letter; for referencing this appendix elsewhere, use \ref{AppendixX}

Write your Appendix content here.
